# Supplementary material for: Multi-Agent Systems for Robotic Autonomy with LLMs
Source: arXiv:2505.05762 source file (2025-05-09)
Supplement: Supplementary file 1 [file X_suppl.tex]

\clearpage
\setcounter{page}{1}
\maketitlesupplementary

\section{Rationale}
\label{sec:rationale}
Having the supplementary compiled together with the main paper means that:
\begin{itemize}
\item The supplementary can back-reference sections of the main paper, for example, we can refer to \cref{sec:intro};
\item The main paper can forward reference sub-sections within the supplementary explicitly (e.g. referring to a particular experiment); 
\item When submitted to arXiv, the supplementary will already included at the end of the paper.
\end{itemize}
To split the supplementary pages from the main paper, you can use \href{https://support.apple.com/en-ca/guide/preview/prvw11793/mac#:~:text=Delete%20a%20page%20from%20a,or%20choose%20Edit%20%3E%20Delete).}{Preview (on macOS)}, \href{https://www.adobe.com/acrobat/how-to/delete-pages-from-pdf.html#:~:text=Choose%20%E2%80%9CTools%E2%80%9D%20%3E%20%E2%80%9COrganize,or%20pages%20from%20the%20file.}{Adobe Acrobat} (on all OSs), as well as \href{https://superuser.com/questions/517986/is-it-possible-to-delete-some-pages-of-a-pdf-document}{command line tools}.

\subsection{Paper ID}
Make sure that the Paper ID from the submission system is visible in the version submitted for review (replacing the ``*****'' you see in this document).
If you are using the \LaTeX\ template, \textbf{make sure to update paper ID in the appropriate place in the tex file}.

When you cite multiple papers at once, please make sure that you cite them in numerical order like this \cite{Alpher02,Alpher03,Alpher05,Authors14b,Authors14}.

By incorporating LLMs into the memory, communication,
and planning modules, the framework enables agents
to utilize natural language to improve both understanding
and execution of cooperative tasks. Kannan et al. [64] introduced
SMART-LLM, a framework that integrated LLM
with multi-agent robot task planning to translate high-level
instructions into executable strategies for robot teams.

\begin{figure}[t]
  \centering
  \fbox{\rule{0pt}{2in} \rule{0.9\linewidth}{0pt}}
   \caption{Example of caption.
   It is set in Roman so that mathematics (always set in Roman: $B \sin A = A \sin B$) may be included without an ugly clash.}
   \label{fig:onecol}
\end{figure}
